# Supplementary material for: Tellurization of Pd(111): absence of PdTe$_2$ but formation of a TePd$_2$ surface alloy
Source: arXiv:2403.03564 ancillary file (2024-03-06)

## Geometry

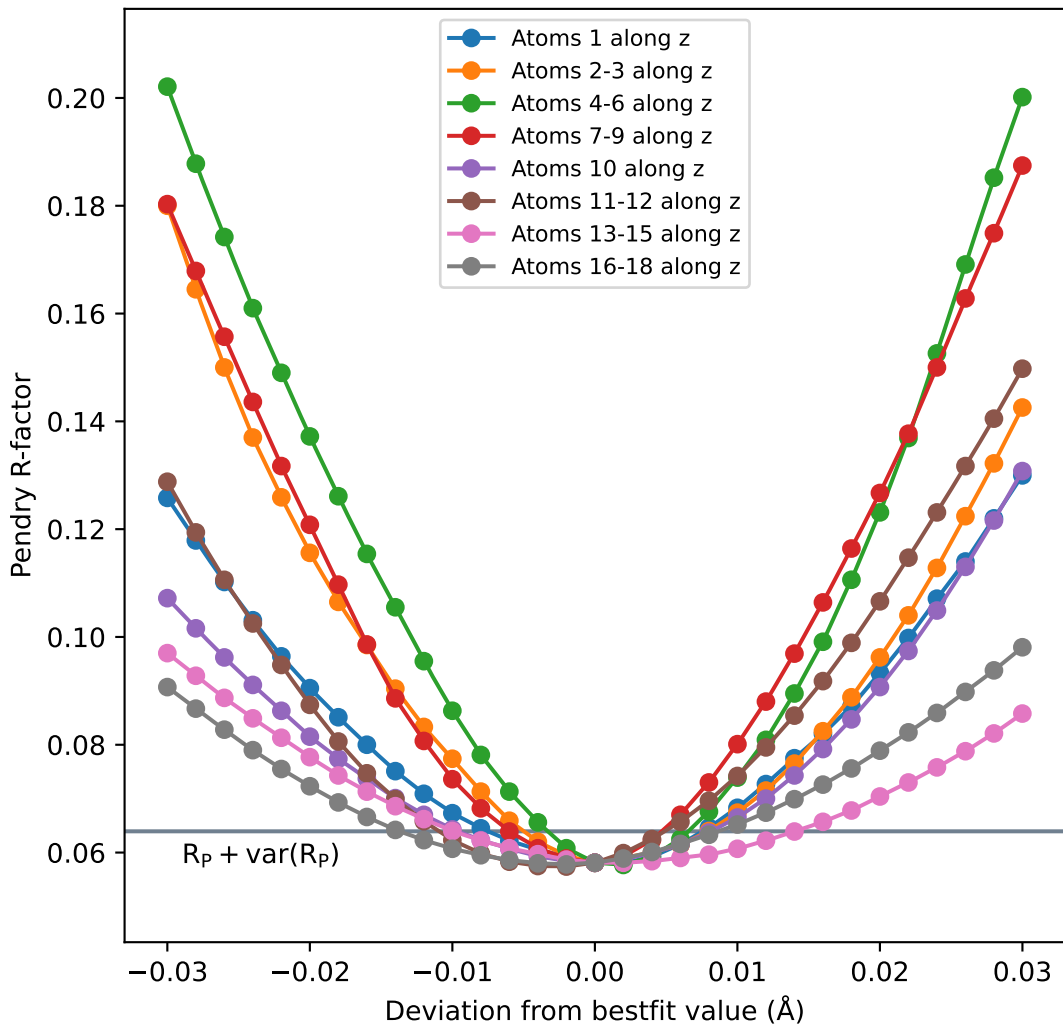

# Geometry

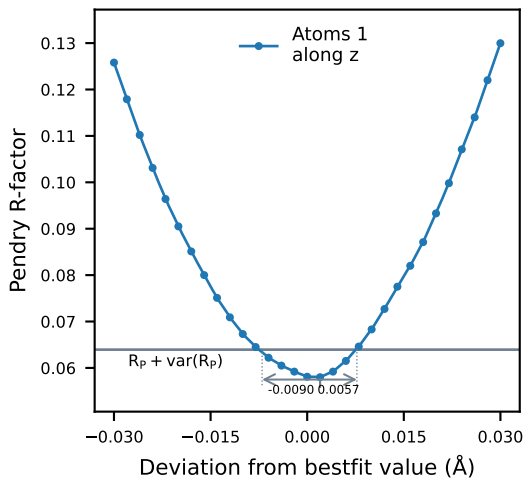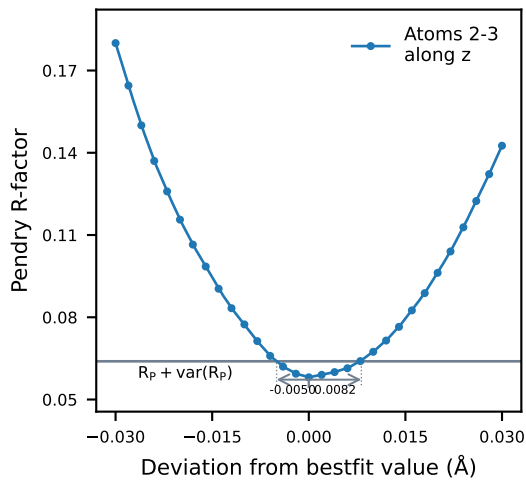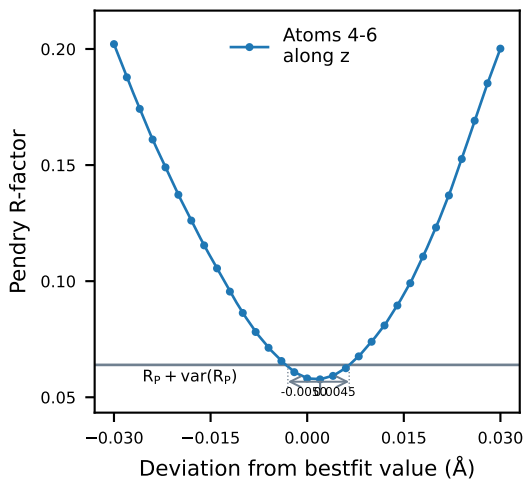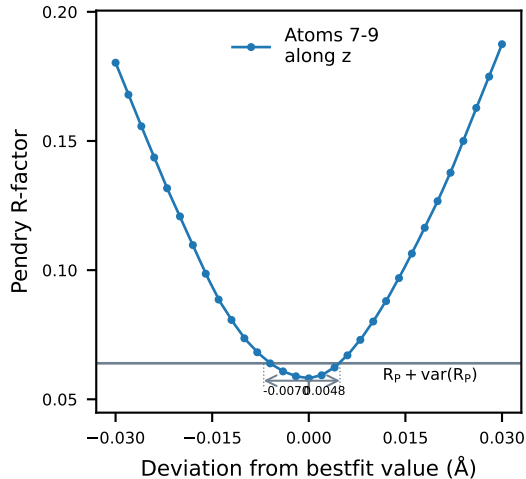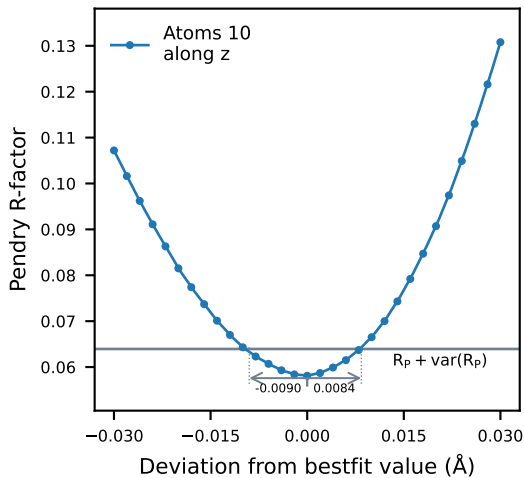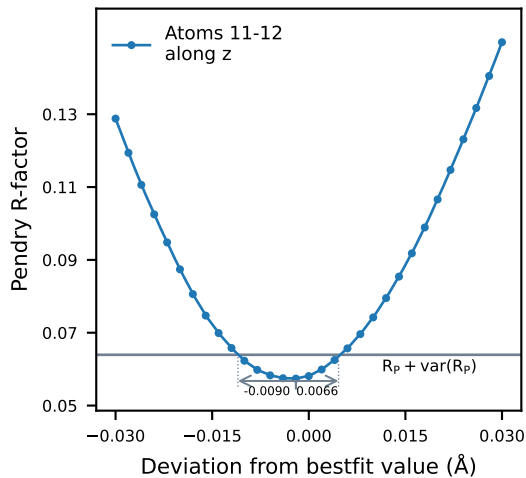

# Geometry

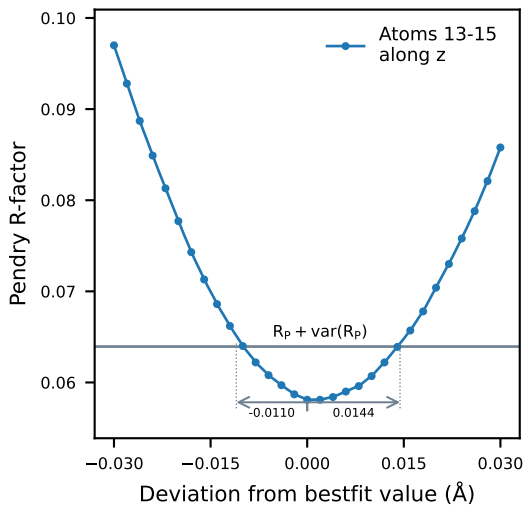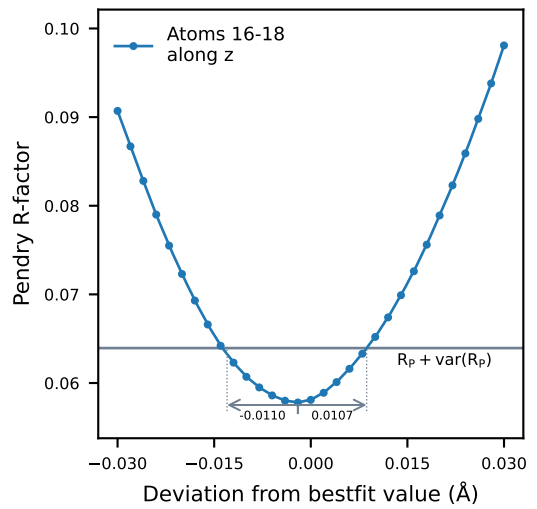

## Geometry

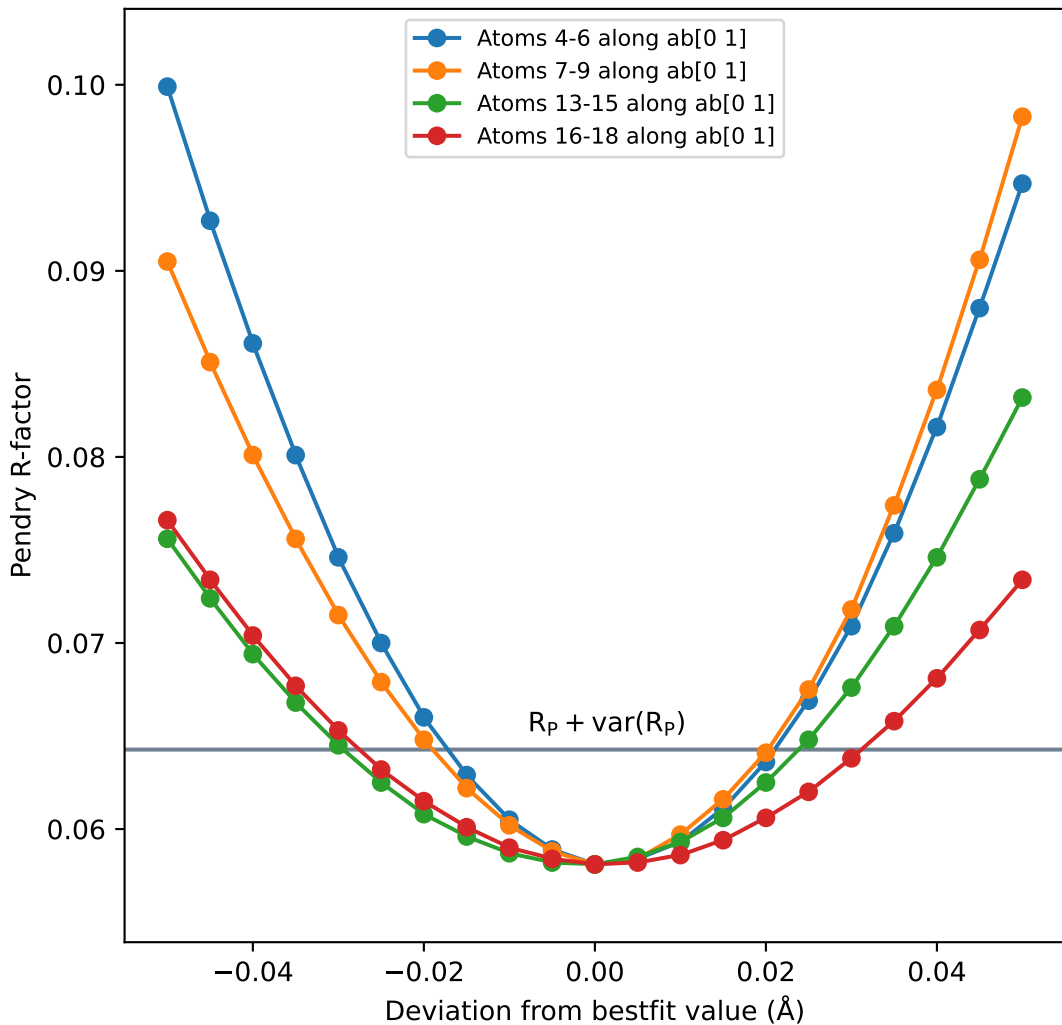

# Geometry

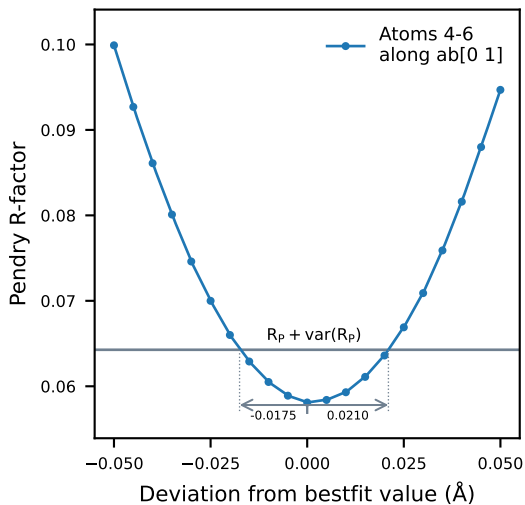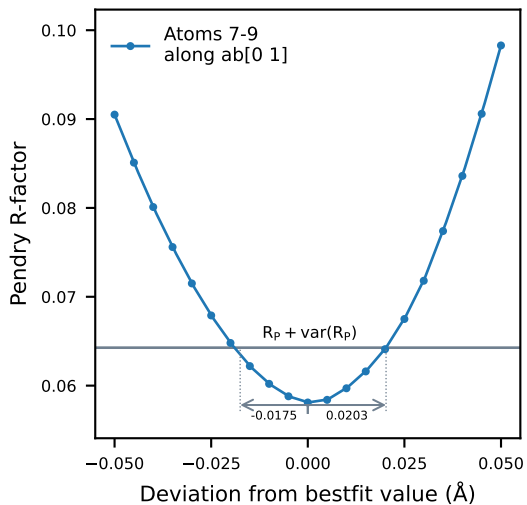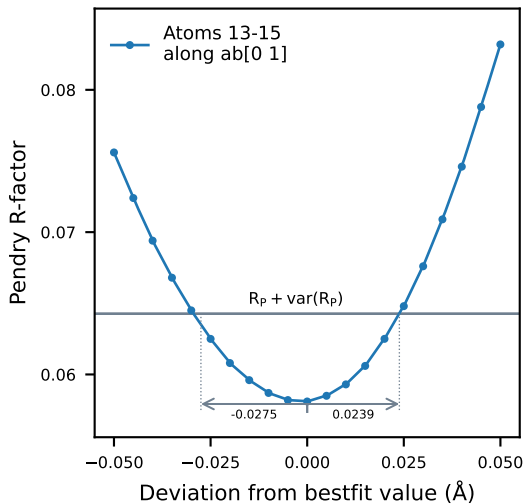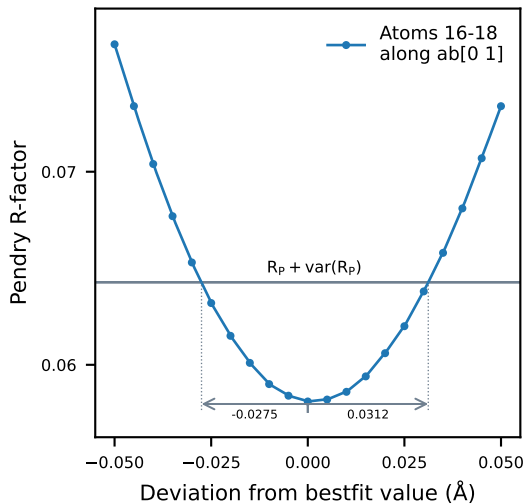

# Vibrational amplitudes

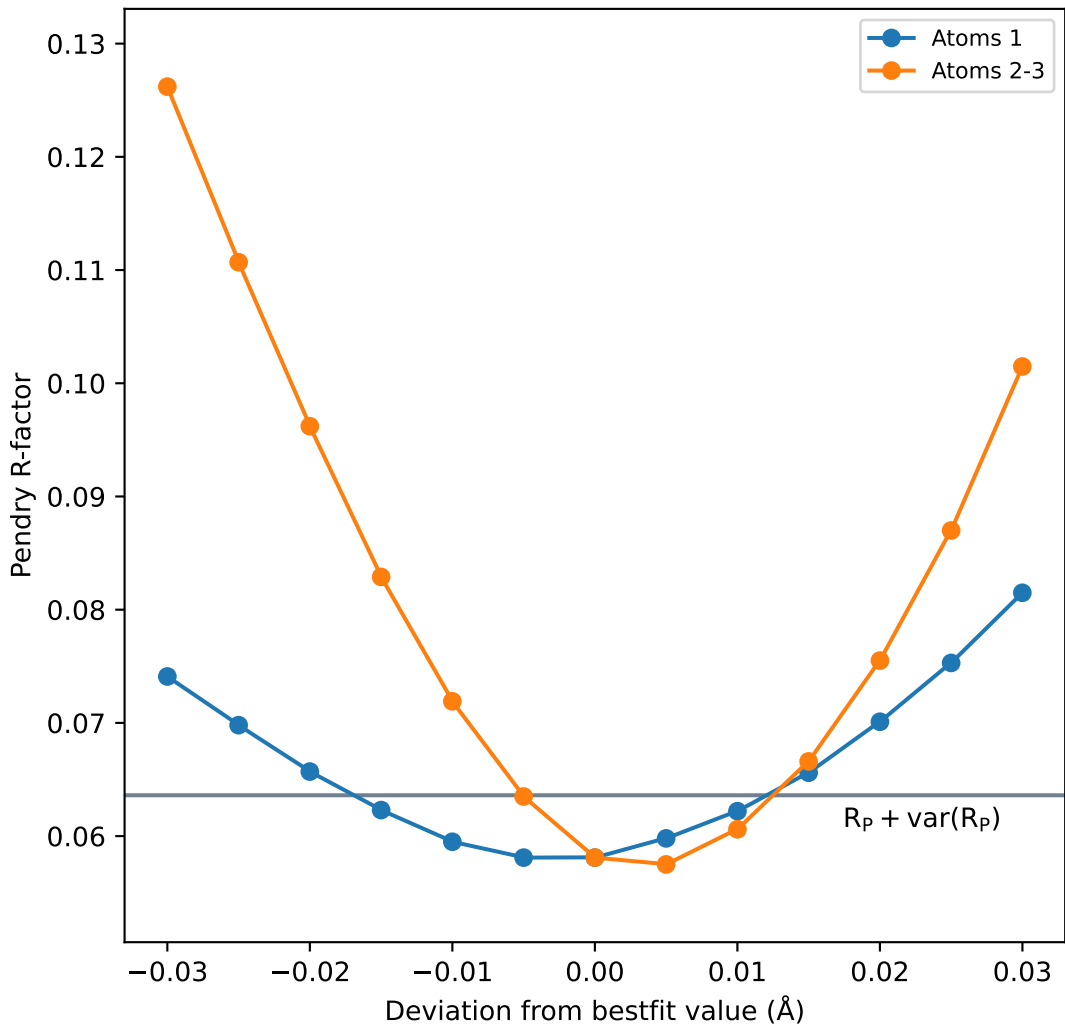

# Vibrational amplitudes

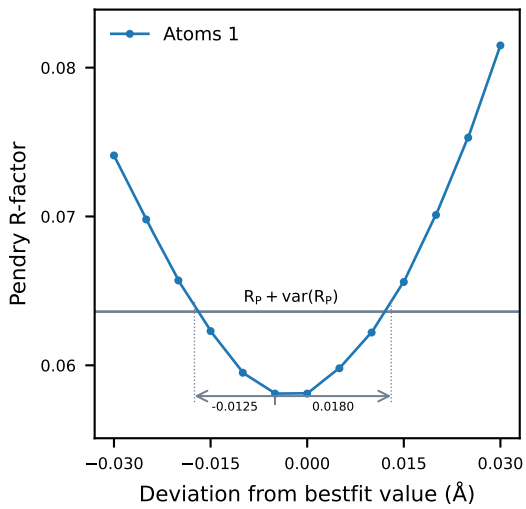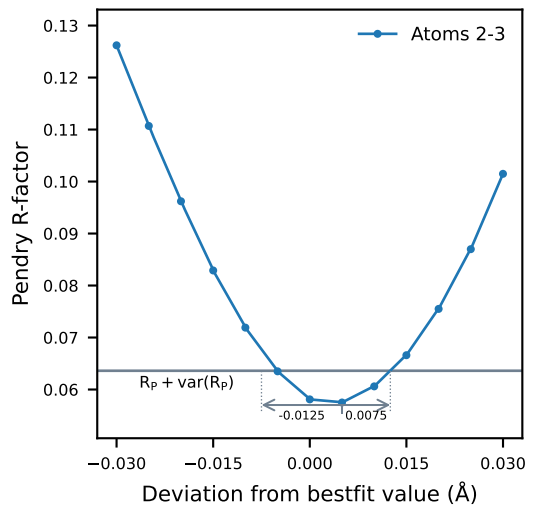

Supplement: Supplementary file 1 [file Errors.pdf]
