# Supplementary material for: Tellurization of Pd(111): absence of PdTe$_2$ but formation of a TePd$_2$ surface alloy
Source: arXiv:2403.03564 ancillary file (2024-03-06)
Supplement: Supplementary file 2 [file Rfactor_plots.pdf]

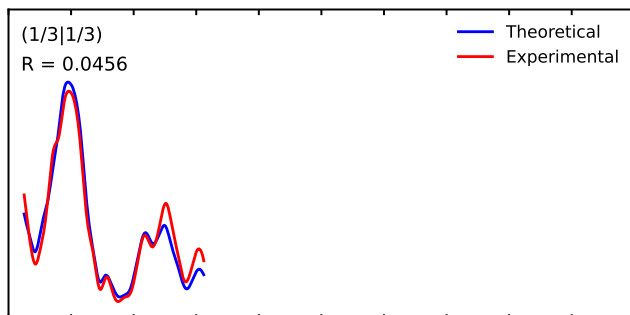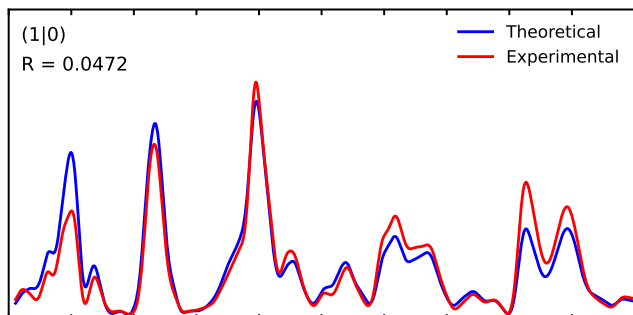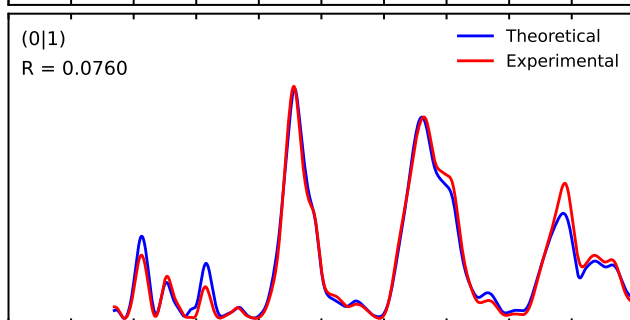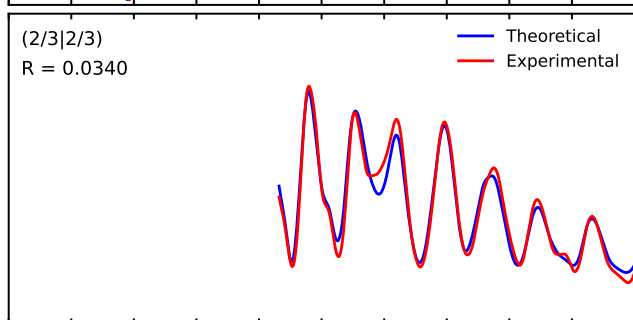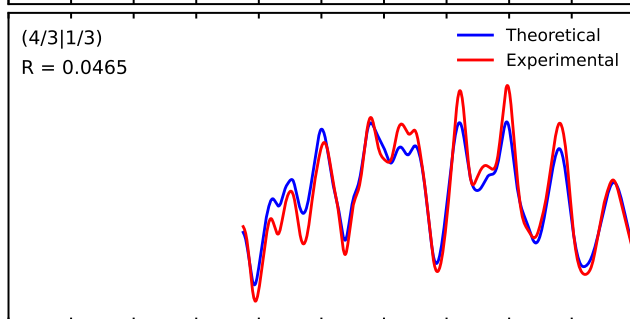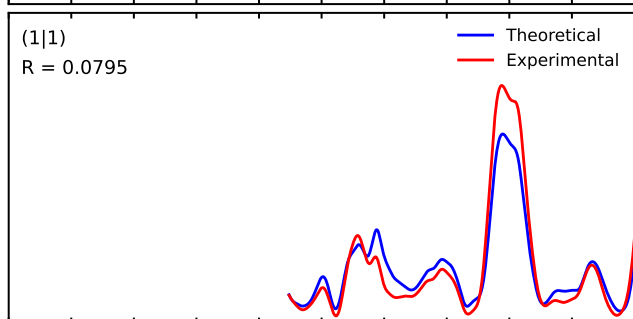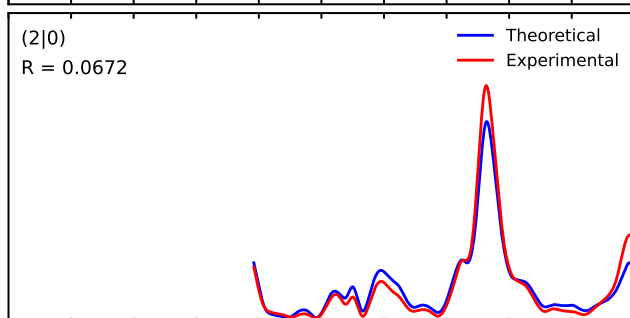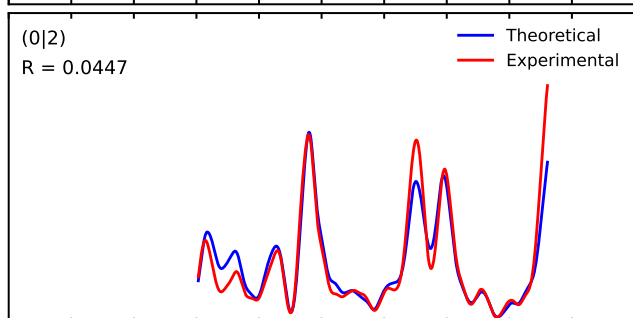

Energy (eV)

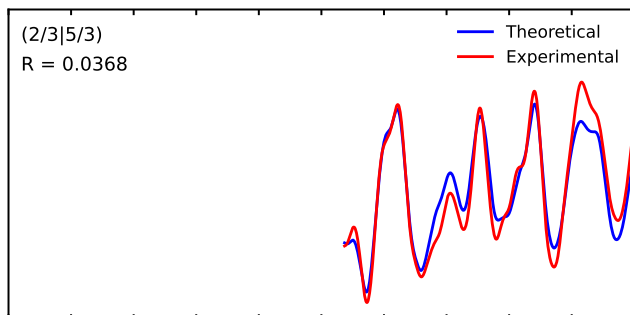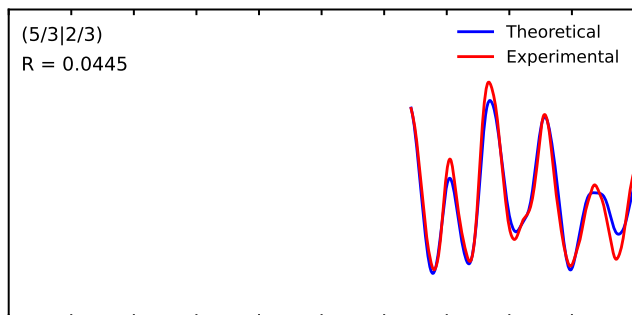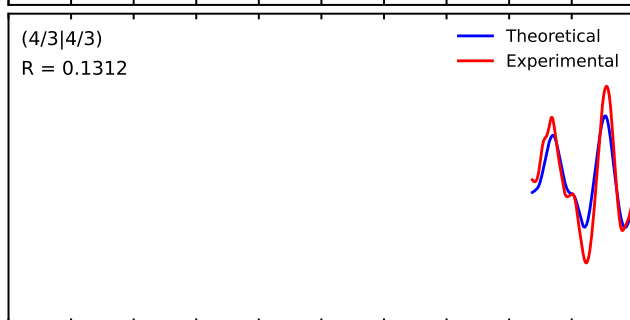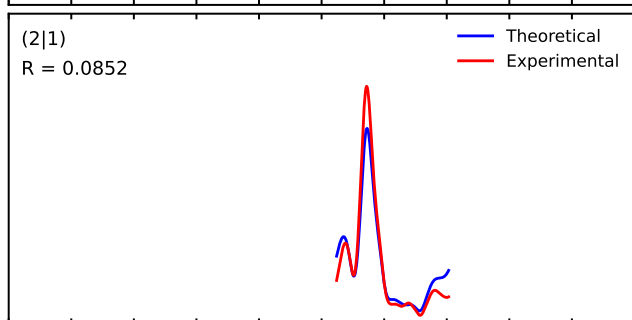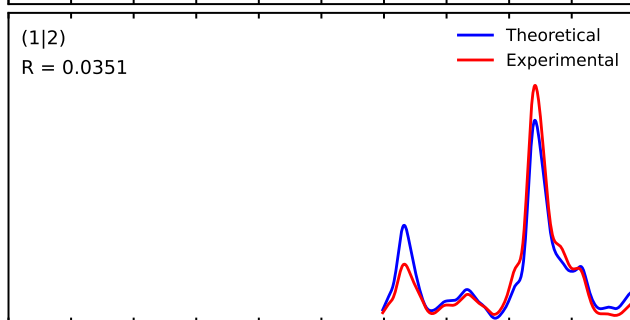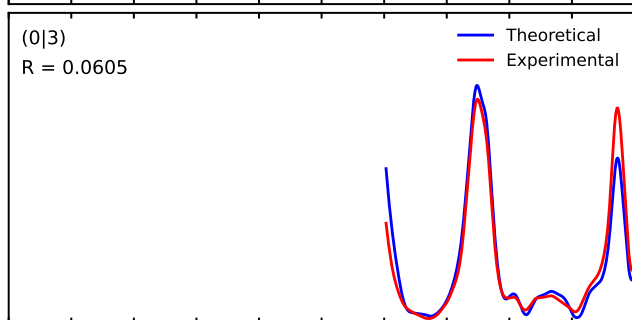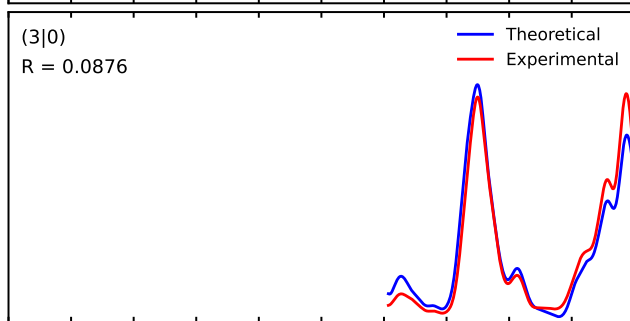

100 150 200 250 300 350 400 450 500 550 600  
Energy (eV)
